# Supplementary material for: GraVoS: Voxel Selection for 3D Point-Cloud Detection
Source: arXiv:2208.08780 source file (2024-03-14)
Supplement: Supplementary file 1 [file gradients_fig_supp.tex]

\begin{figure*}[!ht]
\centering
\begin{tabular}{cccc}
\subfloat{\includegraphics[width=\imwidth\linewidth]{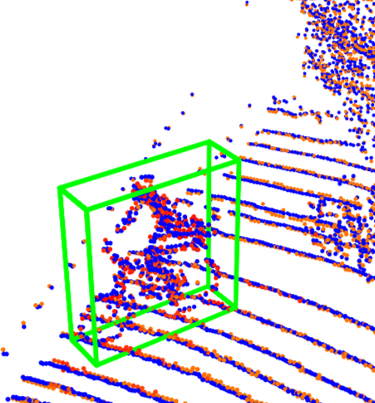}} &
\subfloat{\includegraphics[width=\imwidth\linewidth]{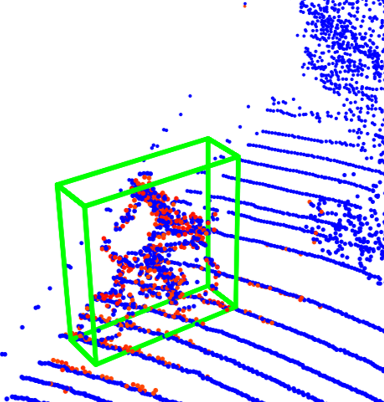}} &
\subfloat{\includegraphics[width=\imwidth\linewidth]{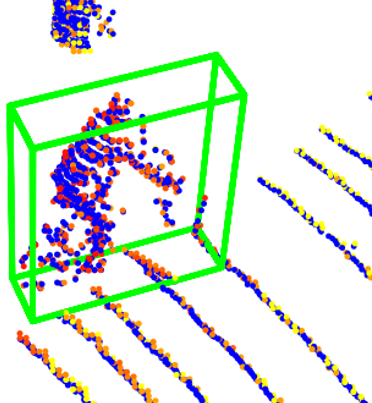}} &
\subfloat{\includegraphics[width=\imwidth\linewidth]{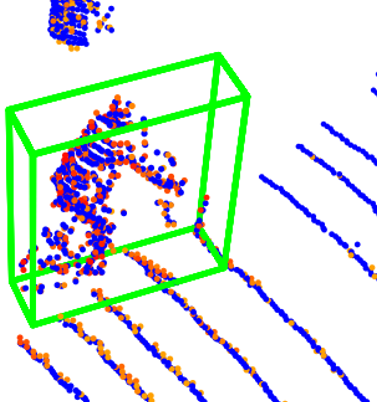}}\\
\subfloat{\includegraphics[width=\imwidth\linewidth]{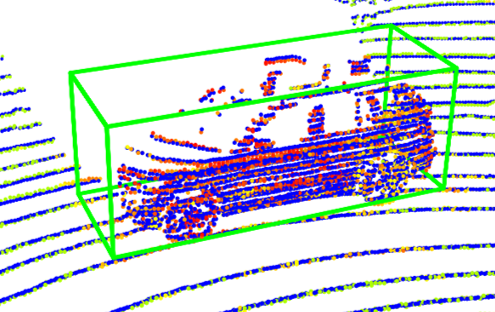}} &
\subfloat{\includegraphics[width=\imwidth\linewidth]{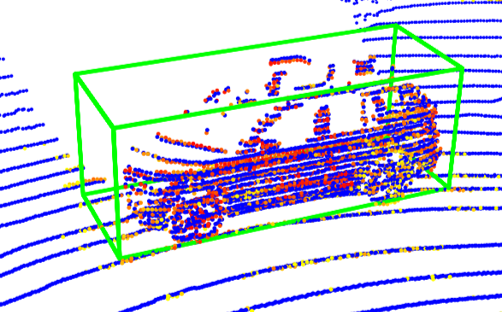}} &
\subfloat{\includegraphics[width=\imwidth\linewidth]{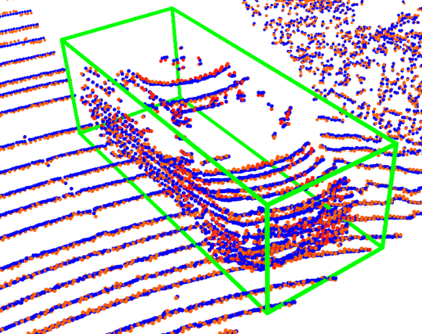}} &
\subfloat{\includegraphics[width=\imwidth\linewidth]{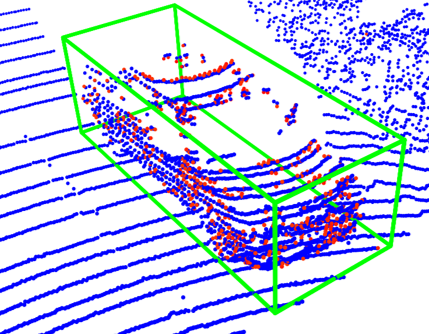}}\\
\subfloat{\includegraphics[width=\imwidth\linewidth]{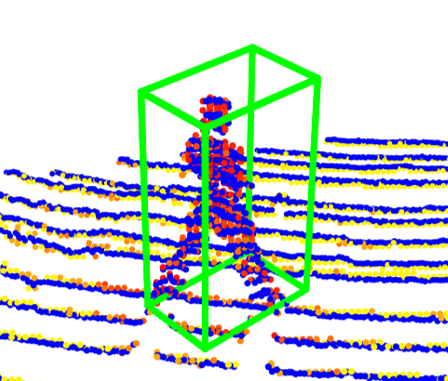}} &
\subfloat{\includegraphics[width=\imwidth\linewidth]{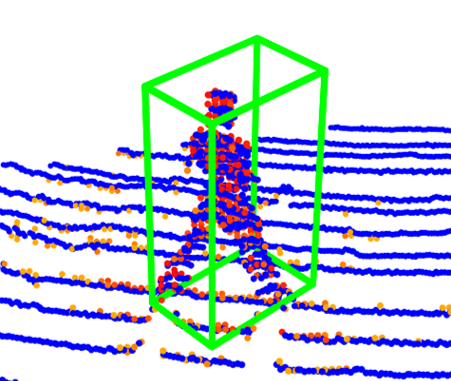}} &
\subfloat{\includegraphics[width=\imwidth\linewidth]{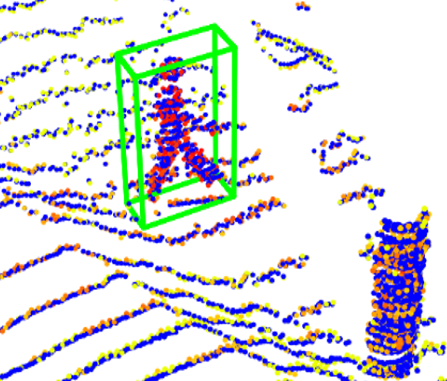}} &
\subfloat{\includegraphics[width=\imwidth\linewidth]{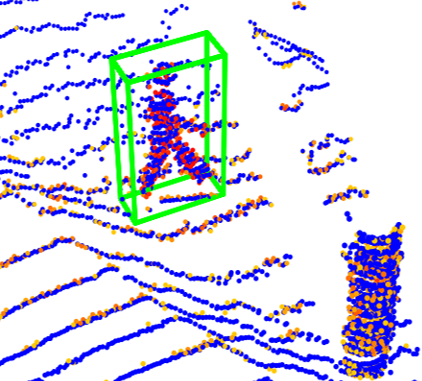}}\\
\subfloat{\includegraphics[width=\imwidth\linewidth]{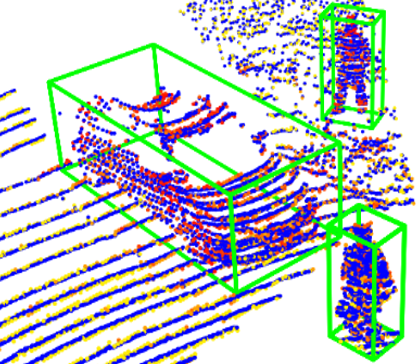}} &
\subfloat{\includegraphics[width=\imwidth\linewidth]{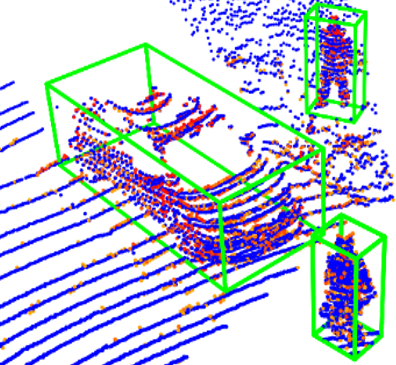}} &
\subfloat{\includegraphics[width=\imwidth\linewidth]{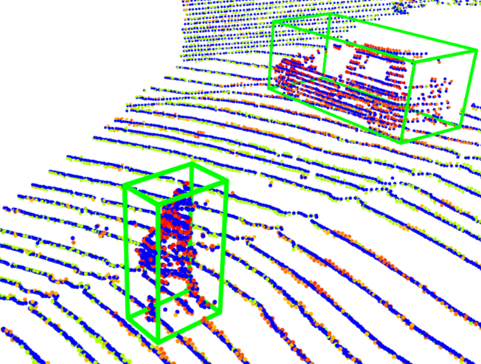}} &
\subfloat{\includegraphics[width=\imwidth\linewidth]{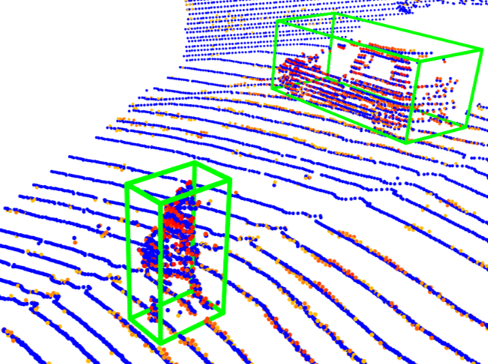}}\\
(a) Gradinent magnitudes & (b) Final subset $S^{mf}$ & (a) Gradinent magnitudes & (b) Final subset $S^{mf}$
\end{tabular}
\caption{\textbf{Gradient-based voxel selection visualization.} 
In each row we have two pairs of images (left pair and right pair). 
Each pair represents the gradient magnitude (a) along with the final choice subset gradient magnitudes (b). 
The top row depicts the {\em Cyclist} class, where in the second and third rows we have the {\em Car} and {\em Pedestrian} classes respectively. 
At the bottom row we have two sub-scenes with multiple classes. 
The magnitude of the gradients is depicted as a color-map from blue to red representing low to high values.
}
\label{fig:gravos_gradient_mag_supp}
\end{figure*}
