# Supplementary material for: GraVoS: Voxel Selection for 3D Point-Cloud Detection
Source: arXiv:2208.08780 source file (2024-03-14)
Supplement: Supplementary file 2 [file sota_comparison_bev_supp.tex]

\begin{table*}[t]
    \centering
    \small
    \begin{tabular}{|l |c c c| c c c| c c c| c c c c | c|}
    \hline
         & \multicolumn{3}{c}{\em Car}  & \multicolumn{3}{|c}{\em Cyclist} & \multicolumn{3}{|c|}{\em Pedestrian} & \multicolumn{4}{c|}{Average} \\
        Method & \multicolumn{1}{c}{Easy} & \multicolumn{1}{c}{Mod.} & \multicolumn{1}{c|}{Hard} & \multicolumn{1}{c}{Easy} & \multicolumn{1}{c}{Mod.} & \multicolumn{1}{c|}{Hard} & \multicolumn{1}{c}{Easy} & \multicolumn{1}{c}{Mod.} & \multicolumn{1}{c|}{Hard} &  
        \multicolumn{1}{c}{\em Car} & \multicolumn{1}{c}{\em Cyc.} & \multicolumn{1}{c}{\em Ped.}  & \multicolumn{1}{c|}{All} \\ \hline
        \hline
        SECOND \cite{second} & 92.30 & \textbf{89.68} & \textbf{87.51} & 87.87 & \textbf{70.91} & 66.57 & 60.94 & 55.73 & 51.56 & 89.83 & 75.12 & 56.08 & 73.67 \\
        Ours & \textbf{92.86} & 89.62 & 87.26 & \textbf{89.02} & 70.88 & \textbf{66.77} & \textbf{62.23} & \textbf{56.78} & \textbf{52.63} & \textbf{89.91} & \textbf{75.56} & \textbf{57.21} & \textbf{74.23} \\ 
        Error reduction & 7.27 & -0.58 & -2.00 & 9.48 & -0.10 & 0.60 & 3.30 & 2.37 & 2.21 & 0.79 & 1.77 & 2.57 & 2.13 \\
        \hline
        Voxel R-CNN \cite{voxelrcnn} & \textbf{95.96} & 91.43 & \textbf{90.70} & 93.63 & 76.09 & \textbf{72.58} & 69.97 & 63.60 & 59.04 & \textbf{92.70} & 80.77 & 64.20 & 79.22 \\ 
        Ours & \textbf{95.96} & \textbf{91.96} & 89.49 & \textbf{94.47} & \textbf{76.32} & 71.60 & \textbf{72.37} & \textbf{66.24} & \textbf{60.31} & 92.47 & \textbf{80.80} & \textbf{66.31} & \textbf{79.86} \\ 
        Error reduction & 0	& 6.18 & -13.01 & 13.19 & 0.96 & -3.57 & 7.99 & 7.25 & 3.10 & -3.15 & 0.16 & 5.89 & 3.08 \\
        \hline
        Part-$A^2$ \cite{parta2} & \textbf{92.89} & \textbf{90.14} & \textbf{88.17} & 91.19 & 75.42 & 70.97 & 68.31 & 61.70 & 57.33 & \textbf{90.40} & 79.19 & 62.45 & 77.35 \\
        Ours & 92.85 & 90.07 & 88.13 & \textbf{93.13} & \textbf{75.91} & \textbf{72.68} & \textbf{68.51} & \textbf{62.40} & \textbf{58.04} & 90.35 & \textbf{80.57} & \textbf{62.98} & \textbf{77.97} \\ 
        Error reduction & -0.56 & -0.71 & -0.34 & 22.02 & 1.99 & 5.89 & 0.63 & 1.83 & 1.66 & -0.52 & 6.63 & 1.41 & 2.74 \\
        \hline
        CenterPoint \cite{yin2021center} & \textbf{92.26} & \textbf{89.30} & \textbf{88.10} & 83.84 & 66.40 & 63.05 & 61.26 & 58.08 & 54.83 & \textbf{89.89} & 71.10 & 58.06 & 73.01 \\ 
        Ours & 91.91 & 88.90 & 88.00 & \textbf{85.68} & \textbf{68.22} & \textbf{64.51} & \textbf{62.32} & \textbf{59.19} & \textbf{55.80} & 89.60 & \textbf{72.80} & \textbf{59.10} & \textbf{73.84} \\ 
        Error reduction & -4.52 & -3.74 & -0.84 & 11.39 & 5.42 & 3.95 & 2.74 & 2.65 & 2.15 & -2.87 & 5.88 & 2.48 & 3.08 \\
        \hline
    \end{tabular}
\vspace{1pt}
\caption{{\bf Performance on the Bird Eye View (BEV) detection  benchmark. }
Similarly to \tabref{tab:sota_comparison}, our method is beneficial for all four detectors.
}
\label{tab:sota_comparison_bev_supp}
\end{table*}
